# Supplementary material for: Pathway to Optical-Cycle Dynamic Photonics: Extreme Electron Temperatures in Transparent Conducting Oxides
Source: arXiv:2512.24641 source file (2026-08-21)
Supplement: Supplementary file 1 [file Supplementary.pdf]

# Supplementary Information

## Pathway to Optical-Cycle Dynamic Photonics: Extreme Electron Temperatures in Transparent Conducting Oxides

Jae Ik Choi[1], Vahagn Mkhitaryan[2], Colton Fruhling[2], Jacob B. Khurgin[3],

Alexander V. Kildishev[2], Vladimir M. Shalaev[2], Alexandra Boltasseva[1,2]

[1]School of Materials Engineering, Purdue University, West Lafayette, IN 47907, USA
[2]Elmore Family School of Electrical and Computer Engineering, Purdue University, West Lafayette, IN 47909, USA
[3]Department of Electrical and Computer Engineering, Johns Hopkins University, Baltimore, MD 21218, USA

December 31, 2025

# Contents


**1 Static optical response of the inverse-designed cavity 3**

**2 Time-dependent transmittance modulation 5**

**3 Electron temperature dependent refractive index of TCOs 6**

**4 Two temperature model 8**

**5 Thermionic emission boundary condition at the TCO/Si interface 10**

**6 Femtosecond scale thermalization in the electron acceptor layer 12**

**7 Refractive and absorptive sensitivities of transmittance 14**

**8 Advantages of ENZ pump excitation 15**

**9 Origin of the transmittance oscillation 16**

**10 Spectral tunability of the zero-crossing through angular variation 18**

**11 Absolute transmittance modulation spectrum 20**

**12 Electron temperature-dependent chemical potential and carrier density of the TCO absorber/acceptor layer 21**

**13 Temporal and spectral tunability of $\Delta n/n$ 22**

# 1 Static optical response of the inverse-designed cavity

Here we present the static optical response of the inverse-designed multilayer cavity incorporating 10 nm transparent conducting oxide (TCO) layer. Aluminum-doped zinc oxide (AZO) serves as the representative TCO material. As shown in Figure S1, the absorptance in the ENZ region of the inverse-designed cavity is enhanced by over threefold, compared to a single TCO film with identical carrier concentration and thickness. This enhancement arises from the strong field confinement in the TCO layer due to the cavity resonance. Figure S1(b) presents the simulated field intensity distribution inside the single TCO on glass and inverse-designed cavity. While the single TCO on glass shows an 8-fold larger field intensity relative to free space, the cavity-incorporated TCO layer achieves over 25-fold enhancement. This enhanced field intensity leads to over 3-fold increase in absorptance in the cavity-incorporated TCO layer and results in an electron temperature exceeding the Fermi temperature within the film.

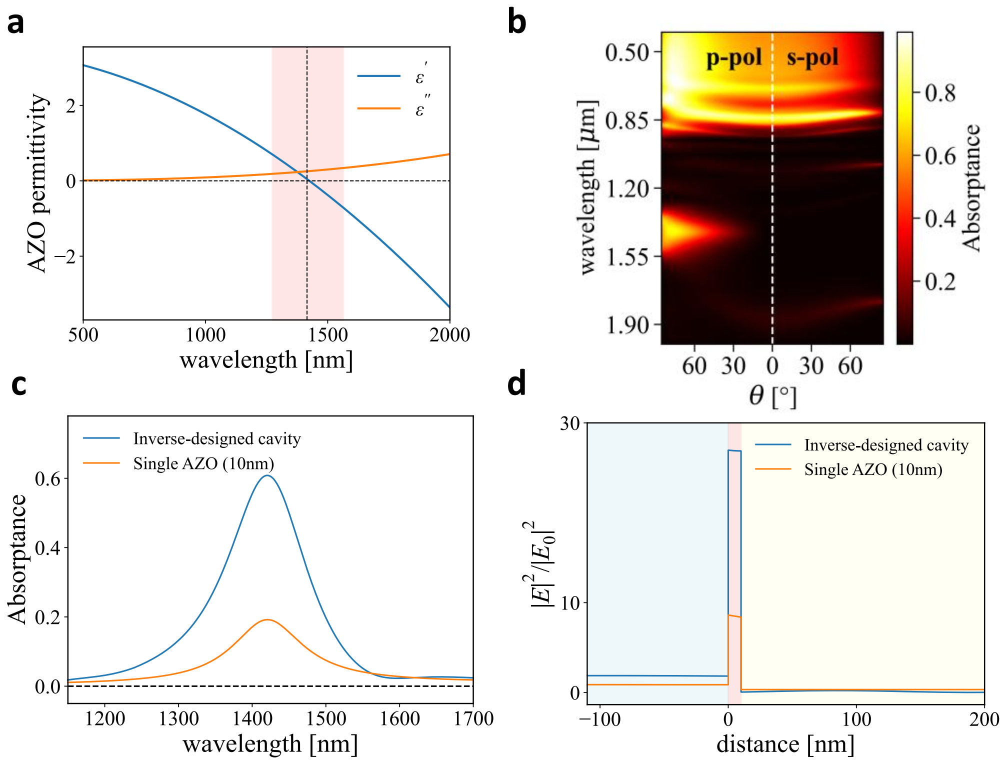


Figure S1: **Static optical response of the inverse-designed cavity.** **a**, Complex permittivity of the aluminum-doped zinc oxide (AZO) layer used in the inverse-designed cavity, showing the epsilon-near-zero (ENZ) region near 1425 nm, highlighted in red. **b**, Simulated absorptance spectrum over incident angle and polarization, showing strong absorption near the ENZ region for p-polarized light. **c**, Absorptance of the TCO layer in the inverse-designed cavity compared to that of an identical 10-nm TCO film on glass at 60° incidence, showing more than a threefold enhancement in the cavity structure. **d**, Relative field intensity within the inverse-designed cavity and the single TCO film on glass, illuminated under ENZ pump (1425 nm) at 60° incidence.

## 2 Time-dependent transmittance modulation

The transmittance modulation of the multilayer structure is strongly dependent on the complex permittivity change of the active nonlinear material. In the inverse-designed cavity, the overall modulation is governed by the modulation of the TCO layer, which has several orders of magnitude stronger nonlinear response compared to that of the Si layers [1, 2]. The time-dependent transmittance modulation is calculated through Eq. S1, originating from a first-order expansion of the transmittance response with respect to changes in the complex permittivity $\varepsilon = \varepsilon' + i\varepsilon''$. Using the chain rule, the time-dependent modulation of the logarithmic transmission can be written as:

$$\ln\left(\frac{T_{\mathrm{mod}}(\lambda,\tau)}{T(\lambda)}\right) = \frac{\partial \ln T(\lambda)}{\partial \varepsilon'}\Delta\varepsilon(\tau)' + \frac{\partial \ln T(\lambda)}{\partial \varepsilon''}\Delta\varepsilon''(\tau). \tag{S1}$$

This is derived from integrating the transmittance variation obtained from the chain rule (Eq. S2).

$$\int \delta \ln T(\lambda,\tau) = \int \left.\frac{\partial \ln T(\lambda)}{\partial \varepsilon'}\right|_{\varepsilon_0} \delta\varepsilon'(\tau) + \int \left.\frac{\partial \ln T(\lambda)}{\partial \varepsilon''}\right|_{\varepsilon_0} \delta\varepsilon''(\tau), \tag{S2}$$

This approximation assumes that the spectral derivatives of transmittance with respect to $\varepsilon'$ and $\varepsilon''$ do not vary significantly over the course of the transient response, allowing them to be treated as constants during integration. While this assumption is justified for structures with relatively broad resonances, it breaks down in extremely high-$Q$ cavities, where even small changes in permittivity can induce pronounced spectral shifts. In our case, the cavity-enhanced ENZ resonance benefits from the intrinsically broad absorption of ENZ materials, ensuring the validity of this framework. Notably, this approximation has been demonstrated to have excellent agreement with experiments in closely related structures such as Tamm plasmon cavities [3, 4].

# 3 Electron temperature dependent refractive index of TCOs

TCOs exhibit a non-parabolic conduction band which is described by a modified energy–momentum relation (Eq. S3). The parameter $C = 0.27$ eV$^{-1}$ characterizes the degree of non-parabolicity, and the effective electron mass at the conduction band minimum is $m^* = 0.24m_e$, where $m_e$ is the free electron mass. $E$ and $k$ correspond to the electron energy and wavevector.

$$\frac{\hbar^2 k^2}{2m^*} = E + CE^2, \tag{S3}$$

From this dispersion relation, the density of states $g(E)$ is derived as:

$$g(E) = \frac{\sqrt{2}}{\pi^2}\left(\frac{m^*}{\hbar^2}\right)^{3/2}\left[(1+CE)^{1/2}(1+2CE)\right], \tag{S4}$$

which effectively captures the deviation from a parabolic band by including higher-order terms.

This density of states is used to calculate the electron temperature-dependent chemical potential, which in turn determines the plasma frequency and optical loss. Together, these quantities govern the complex permittivity through the Drude model (Eq. S5).

$$\epsilon(\omega) = \epsilon_\infty - \frac{\omega_p^2}{\omega^2 + i\Gamma\omega} \tag{S5}$$

Here, $\epsilon(\omega)$ is the complex permittivity, $\epsilon_\infty$ represents the high-frequency contribution from bound electrons, $\omega_p = \sqrt{ne^2/(m^*\varepsilon_0)}$ defines the plasma frequency, and $\Gamma = 1/\tau$ denotes the damping rate associated with electron scattering with phonons, impurities, grain boundaries, and surface roughness. Both $\omega_p$ and $\Gamma$ vary with electron temperature as heating alters carrier distribution and scattering dynamics, leading to a time-dependent evolution of the material's permittivity.

The electron temperature–dependent plasma frequency (Eq. S6) in a non-parabolic conduction band deviates from the conventional expression $\omega_p = \sqrt{n_e e^2/(\varepsilon_0 m^*)}$ and is derived from the linearized Boltzmann transport equation [1, 5, 6].

$$\omega_{\mathrm{p}}^2(T_{\mathrm{e}}) = \frac{e^2}{3m^*\varepsilon_0\pi^2}\int_0^\infty \frac{\mathrm{d}E}{1+2CE}\left(\frac{2m^*}{\hbar^2(E+CE^2)}\right)^{3/2}\left(-\frac{\partial f_{\mathrm{FD}}(E,\mu(T_{\mathrm{e}}),T_{\mathrm{e}})}{\partial E}\right), \tag{S6}$$

$$n_e = \int_0^\infty f_{\mathrm{FD}}(E,\mu(T_{\mathrm{e}}),T_{\mathrm{e}})g(E)\,\mathrm{d}E, \tag{S7}$$

Here, $\omega_p(T_e)$ is the electron temperature-dependent plasma frequency, and $f_{\mathrm{FD}}$ is the Fermi-Dirac distribution, $\mu(T_e)$ is the chemical potential, and $g(E)$ is the density of states. In TCOs, the downward shift in chemical potential $\mu(T_e)$ is much larger compared to the noble metals, leading to a correspondingly more pronounced redistribution of carriers. Other parameters include the non-parabolicity parameter $C$ from the $E-k$ relation, the elementary charge $e$, electron effective mass $m^*$, permittivity of free space $\varepsilon_0$, and carrier density $n_e$. The last term in Eq. S6 determines the strength of thermal broadening, which is substantially larger in TCOs compared to noble metals due to the lower carrier density.

The Drude damping $\Gamma$ in Eq. S8 incorporates electron scattering from phonons, impurities, grain boundaries, and surface roughness.

$$\Gamma(T_{\mathrm{e}}) = \frac{\omega^2}{4\pi^2\omega_{\mathrm{p}}(T_{\mathrm{e}})}\left[1+\left(\frac{2\pi k_{\mathrm{B}}T_{\mathrm{e}}}{\hbar\omega}\right)^2\right], \tag{S8}$$

$\Gamma$ is strongly dependent on the electron temperature and plays a central role in shaping the optical response under high electron temperatures. Because the electron scattering with the surrounding phonon, impurities, and defects is highly sensitive to microstructure, its exact functional form generally requires experimental fitting for each material system. In this work, we employ a quadratic dependence to capture the enhanced damping that governs TCO

nonlinearities, which has become an active area of recent interest. When the electron temperature is well below the Fermi temperature $T_F$, the variation in $\Gamma$ is relatively small. In TCOs, however, where $T_e$ rises extremely high, often exceeding the Fermi temperature ($T_F$), $\Gamma$ becomes increasingly dominant in determining the optical response. Here, $k_B$ is the Boltzmann constant, and $\hbar$ is the reduced Planck constant.

By incorporating both the electron temperature-dependent plasma frequency (Eq. S6) and Drude damping (Eq. S8) into the Drude formula (Eq. S5), the electron temperature-dependent refractive index can be obtained as:

$$n(\omega, T_e) = \sqrt{\epsilon(\omega, T_e)} = \sqrt{\epsilon_\infty - \frac{\omega_p(T_e)^2}{\omega^2 + i\omega\Gamma_{ee}(T_e)}}, \tag{S9}$$

# 4 Two temperature model

The electron temperature evolution in TCOs induced by the intraband optical pumping is obtained by solving the coupled Eqs. S10 and S11, known as the two-temperature model (TTM).

$$C_e(T_e)\frac{\partial T_e}{\partial t} = \frac{\partial}{\partial x}\left(\kappa(T_e)\frac{\partial T_e}{\partial x}\right) - g_{ep}(T_e)(T_e - T_l) + H(x) \tag{S10}$$

$$C_l(T_l)\frac{\partial T_l}{\partial t} = g_{ep}(T_e)(T_e - T_l) \tag{S11}$$

Here, $C_e$ denotes the electron heat capacity, $\kappa$ as the thermal conductivity, $g_{ep}$ signifies the coupling between electron and lattice, $T_l$ is the lattice temperature, and $H(x)$ is the pump-induced heat source. The pump pulse is modeled as a Gaussian envelope defined by its temporal width and central wavelength. The temporal profile is Fourier transformed into the frequency domain, and the transfer matrix method is used to determine the spatially resolved absorbed energy $H(x)$ for each frequency component within the multilayer stack. From this input heat source, the coupled Eqs. S10 and

S11 are solved to obtain the spatio-temporal evolution of the electron temperature. This two-temperature framework is particularly advantageous in multilayer systems, as it retains spatial dependence that is often neglected in simplified treatments. The spatial profile is especially important at TCO–semiconductor interfaces, where electron transport across the junction critically influences the overall transient response. To capture this effect, a thermionic boundary condition is applied at the interface to accurately model thermionic carrier flow and the resulting electron temperature relaxation.

It is essential to account for the electron-temperature dependence of the parameters in the two-temperature model, including the electron heat capacity and electron–phonon coupling coefficient, since these quantities evolve during the electron heating process. The $T_e$-dependent electron heat capacity is calculated using Eq. S12, where $g(E)$ is the density of states (Eq. S4), and $\mu(T_e)$ is the chemical potential obtained from Eq. S7. The lattice heat capacity is taken as a constant, $C_l = 2.54 \times 10^6$ J m$^{-3}$K$^{-1}$, since the lattice temperature changes minimally during a sub-picosecond timescale relative to the huge electron temperature response.

$$C_e(T_e) = \int_0^\infty \frac{\partial f_{FD}(\mu(T_e), T_e)}{\partial T_e} g(E) E \, dE \tag{S12}$$

The electron–phonon coupling coefficient in Eq. S13 governs the hot-electron relaxation through energy transfer to phonons.

$$g_{ep} = \frac{\pi k_B}{\hbar \, g(E_F)} \lambda_{ep} \langle (\hbar\omega_{ph})^2 \rangle \int_{-\infty}^{\infty} g^2(E) \left( -\frac{\partial f_{FD}}{\partial E} \right) dE \tag{S13}$$

Here, $\lambda_{ep}$ is the electron–phonon mass enhancement factor, characterizing the strength of the phonon spectrum, and $\langle (\hbar\omega_{ph})^2 \rangle$ is the second moment of the phonon spectrum, representing the weighted average of phonon energy squared. The product $\lambda_{ep}\langle (\hbar\omega_{ph})^2 \rangle$ is set to $5.25 \times 10^{-4}$, taken from Ref. [1]. The electron temperature dependency of the heat capacity, electron-phonon

coupling coefficient, and chemical potential is plotted in Figure S2.

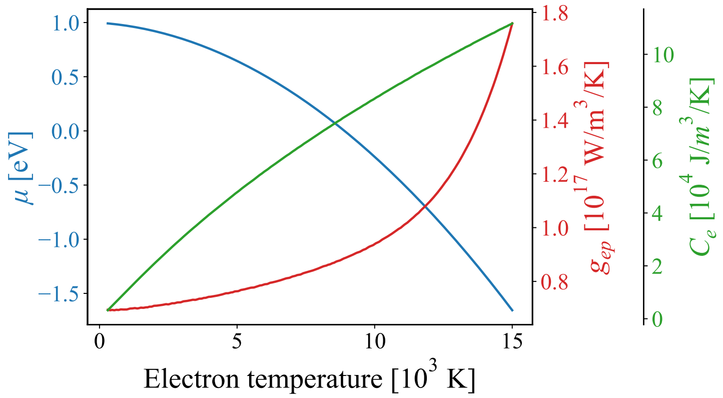


Figure S2: Two-temperature model parameters as a function of electron temperature

## 5 Thermionic emission boundary condition at the TCO/Si interface

The thermionic boundary condition at the TCO/Si interface ($z = z_{\text{interface}}$) describing the heat flux relation involving the space-charge-limited thermionic emission rate $\dot{N}_{sc}$ is incorporated in the two-temperature model to account for accurate hot-electron dynamics within the heterojunction. The boundary condition is given as follows,

$$k_e \left. \frac{\partial T_e}{\partial z} \right|_{z=z_{\text{interface}}} = -(eE_f + e\phi) \left. \dot{N}_{sc} \right|_{z=z_{\text{interface}}}, \tag{S14}$$

where $k_e$ is the electronic thermal conductivity, $e$ is the elementary charge, $E_f$ is the Fermi energy, and $\phi$ denotes the energy barrier in the interface. The emission rate per unit area, $\dot{N}_{sc}$, is determined self-consistently from a modified Richardson–Dushman expression that incorporates both the temperature dependence of the chemical potential $\mu(T_e)$ and the space-charge

potential $\phi_{sc}$.

In the classical Richardson–Dushman formulation, the thermionic emission rate is expressed as:

$$\dot{N}_1 = \frac{A_0}{e} T_e^2 \exp\left(-\frac{e\phi}{k_B T_e}\right), \tag{S15}$$

where $A_0 = 1.2 \times 10^6$ Am$^{-2}$K$^{-2}$ is the Richardson constant, and $k_B$ is Boltzmann's constant. This formulation assumes that the Fermi energy $E_f$ approximates the chemical potential $\mu$ and that the space-charge potential due to electron accumulation is negligible. However, under femtosecond laser excitation, the rapid rise in $T_e$ can lead to a huge deviation of chemical potential from Fermi energy, and a significant space-charge effect, leaving a net positive charge on the interface which perturbs subsequent emission.

To capture these behaviors, a more comprehensive expression for $\dot{N}_{sc}$ is employed:

$$\dot{N}_{sc}(x, y, t) = A(k_B T_e)^2 \exp\left[-\frac{eE_f - \mu(T_e) + e\phi + \phi_{sc}}{k_B T_e}\right], \tag{S16}$$

where $A = 4\pi m^* k_{\mathrm{B}}^2 h^{-3}$, $m$ is the electron mass, $h$ is Planck's constant, and $\phi_{sc}$ is the effective potential due to the space-charge cloud. The electron temperature dynamically evolves during excitation and governs the rate of emission. The space-charge potential is then estimated as:

$$\phi_{sc} \approx \frac{a N_{\mathrm{yield}} e^2}{R_1}, \tag{S17}$$

where $N_{\mathrm{yield}}$ is the total emitted electron yield, $R_1$ is the semi-major axis of the disk, and $a$ is a geometrical factor, often taken as $a = 16/(3\pi\epsilon^2)$ for uniform disks.

Assuming a rectangular pulse with duration $\tau$, the total yield $N_{\mathrm{yield}}$ can

be integrated analytically to yield [7, 8]:

$$N_{\text{yield}} = \frac{k_B T_e}{ae^2/R_1} \log \left[ 1 + C\tau\pi R_2 a e^2 k_B T_e \exp\left( \frac{-eE_f + \mu(T_e) - e\phi}{k_B T_e} \right) \right], \tag{S18}$$

where $R_2$ is the semi-minor axis of the elliptical emission region. This result quantifies the interplay between emission dynamics and space-charge buildup. In the limit where $aN_{\text{yield}}e^2/R_1 \ll k_B T_e$, the space-charge term becomes negligible, and the yield reduces to that of the standard Richardson–Dushman model.

# 6 Femtosecond scale thermalization in the electron acceptor layer

Figure S3(a) and (b) show the electron energy distributions at elevated temperatures for the absorber layer (carrier density of $7.35 \times 10^{26}$ m$^{-3}$) and the acceptor layer ($0.5 \times 10^{26}$ m$^{-3}$), corresponding to the layers highlighted in Figure 4(a) of the main text. As the electron temperature increases, the distributions broaden significantly, extending beyond 5 eV in the absorber and 4 eV in the acceptor at $10^4$ K. Figure S3(c) and (d) present the corresponding Drude damping across probe wavelengths, calculated using Eq. S8. The dotted lines indicate the threshold where the scattering rate reaches $10^{15}$ Hz, corresponding to a femtosecond thermalization time. Moreover, the scattering rate increases with electron energy, as described by Eq. S19, reaching values over two orders of magnitude faster for electrons at 5 eV compared with those near the chemical potential [9].

$$\tau_{\text{ee}}(E) = \tau_0 \frac{\mu^2}{(E-\mu)^2 + (\pi k_B T_{\text{e}})^2}, \tag{S19}$$

$$\text{with} \quad \tau_0 = \frac{128}{\sqrt{3}\pi^2 \omega_p}, \tag{S20}$$

where $E$ is the electron energy, $\mu$ is the chemical potential, and $k_B$ is the Boltzmann constant. Given the substantial population of high-energy electrons in the Fermi tail (Figure S3(a)), carrier injection into the acceptor layer can drive ultrafast thermalization on femtosecond timescales. Therefore, applying the two-temperature model to describe the evolution of electron temperature in the acceptor layer is justified. Previous studies have similarly reported Fermi–Dirac redistribution shortly after population of high-energy states through optical transitions [10, 11]. Notably, femtosecond-scale thermalization has been both theoretically predicted and experimentally observed [12, 13]. Other studies report that the non-thermal electrons could be safely neglected due to an extremely fast thermalization rate from substantially weaker screening compared to noble metals [11, 14]. Moreover, previous studies have shown that the optical response closely follows the behavior of thermal electrons, with non-thermal electron contribution being several orders of magnitude smaller [15]. However, non-thermal electrons may play an important role during the first few femtoseconds of the dynamics and warrant a more detailed theoretical treatment, which is beyond the scope of this work. These frameworks are briefly discussed in the main text.

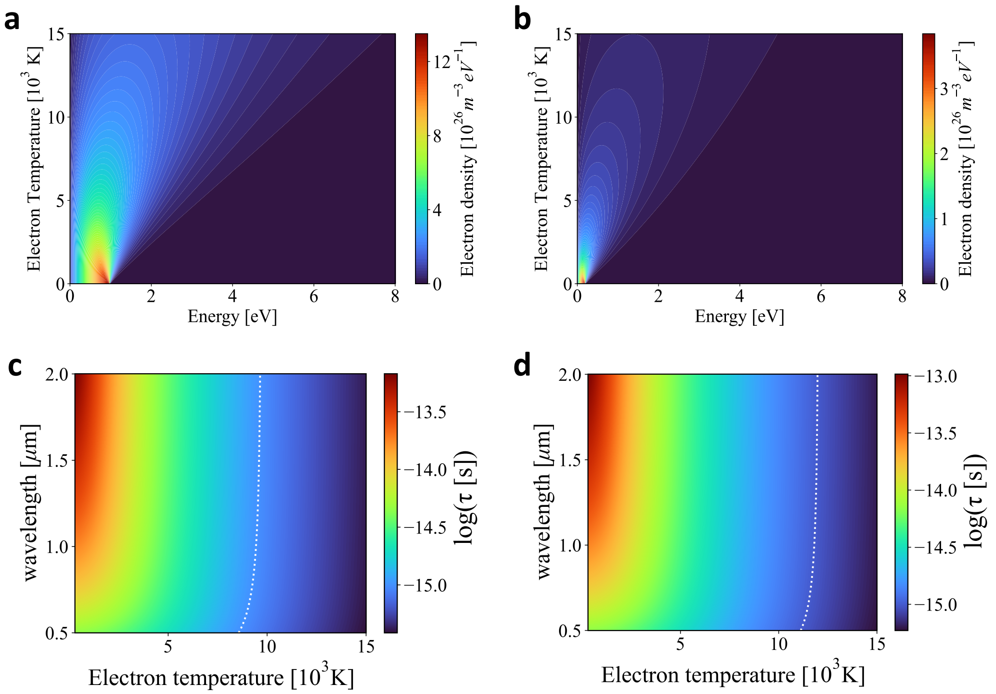


Figure S3: **Electron energy distribution and Drude damping over electron temperature.** **a**, Electron energy distribution in the absorber layer at various electron temperatures, showing substantial amounts of high-energy electron population at elevated electron temperatures. **b**, Electron energy distribution in the acceptor layer as a function of electron temperature. **c**, Calculated Drude damping in the absorber layer across electron temperatures and wavelengths. **d**, Calculated Drude damping in the acceptor layer.

# 7 Refractive and absorptive sensitivities of transmittance

The refractive ($\alpha \equiv \partial \ln \mathcal{T}(\lambda)/\partial\varepsilon'$) and absorptive ($\beta \equiv \partial \ln \mathcal{T}(\lambda)/\partial\varepsilon''$) sensitivities serve as weighting factors that quantify how changes in the real and imaginary components of the permittivity contribute to the overall change

in transmittance. An oscillatory response can arise when the two sensitivities have opposite signs, which occurs in two distinct spectral windows, near the ENZ (right side of the green dotted line, $\alpha > 0$, $\beta < 0$) and off-ENZ (left side of the green dotted line, $\alpha < 0$, $\beta > 0$). Furthermore, wavelength regions where either sensitivity approaches zero correspond to conditions for background-free transmittance [3].

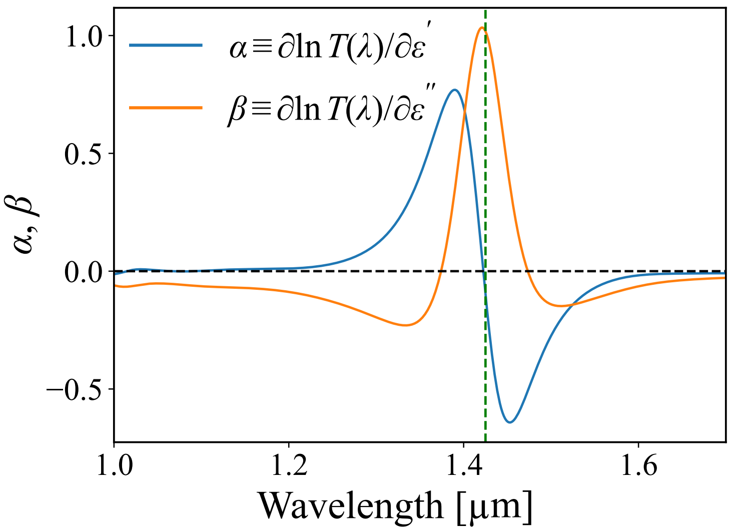


Figure S4: Refractive ($\alpha$) and absorptive ($\beta$) sensitivities of the inverse-designed cavity. The green dotted line at 1425 nm marks the wavelength at which the real permittivity of the TCO crosses zero.

# 8 Advantages of ENZ pump excitation

Here, we demonstrate the strength of ENZ pump excitation in driving oscillatory response in TCO films. The Sommerfeld approximation is employed to reveal the difference compared with the ENZ pump-driven behavior presented in Figure 1(d) of the main text. Figure S5 shows the $\Delta n/n$ of 10 nm TCO film on glass under off-ENZ pump excitation (800 nm). Contrary to the ENZ pump excitation exhibiting a sign reversal in the initial stage, the off-ENZ case shows a single-peaked response with three orders of magnitude

smaller changes due to the significantly lower electron temperature. This highlights the substantial enhancement offered by the ENZ pump excitation. Notably, reaching the same electron temperatures with the off-ENZ pump excitation (800 nm) requires approximately two orders of magnitude higher pump fluence than with ENZ excitation.

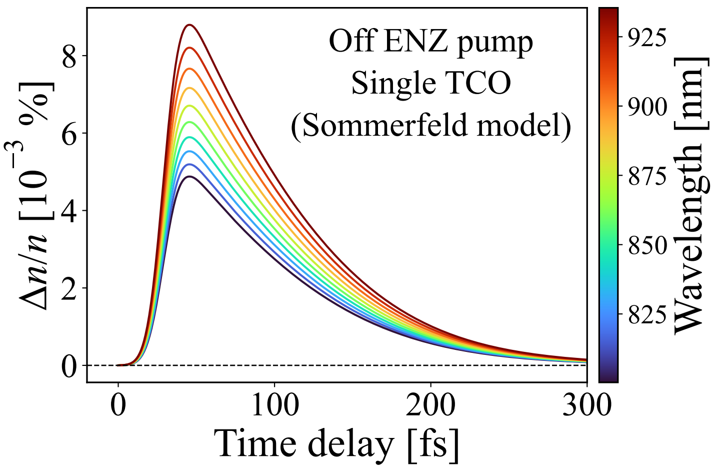


Figure S5: $\Delta n/n$ of 10 nm single TCO film on glass under Off-ENZ pump (800 nm) excitation. A single-peaked response of three orders of magnitude smaller modulation is observed, contrary to the ENZ pump excitation in the main text Figure 1(d).

# 9 Origin of the transmittance oscillation

Figure S6 reveals the origin of the oscillatory transmittance response in the inverse-designed cavity. As shown in Figure S6(a) and (b), the refractive index change of the 10 nm TCO absorber layer exhibits a single-peaked profile, whereas the extinction coefficient oscillates in time. This indicates that the oscillatory transmittance is primarily driven by the variations in the extinction coefficient. Figure S6(c) and (d) further decompose the contribution from real and imaginary permittivity. While both $\Delta\varepsilon'$ and $\Delta\varepsilon''$ increase upon pump excitation, their temporal trends differ—$\Delta\varepsilon'$ shows a single-peaked re-

sponse, whereas $\Delta\varepsilon''$ oscillates. Combined with their respective sensitivity coefficients ($\alpha$, $\beta$), these competing contributions give rise to the overall oscillatory dynamics. The refractive and absorptive terms responsible for the transmittance oscillation near the ENZ region are shown in Figure S6(d).

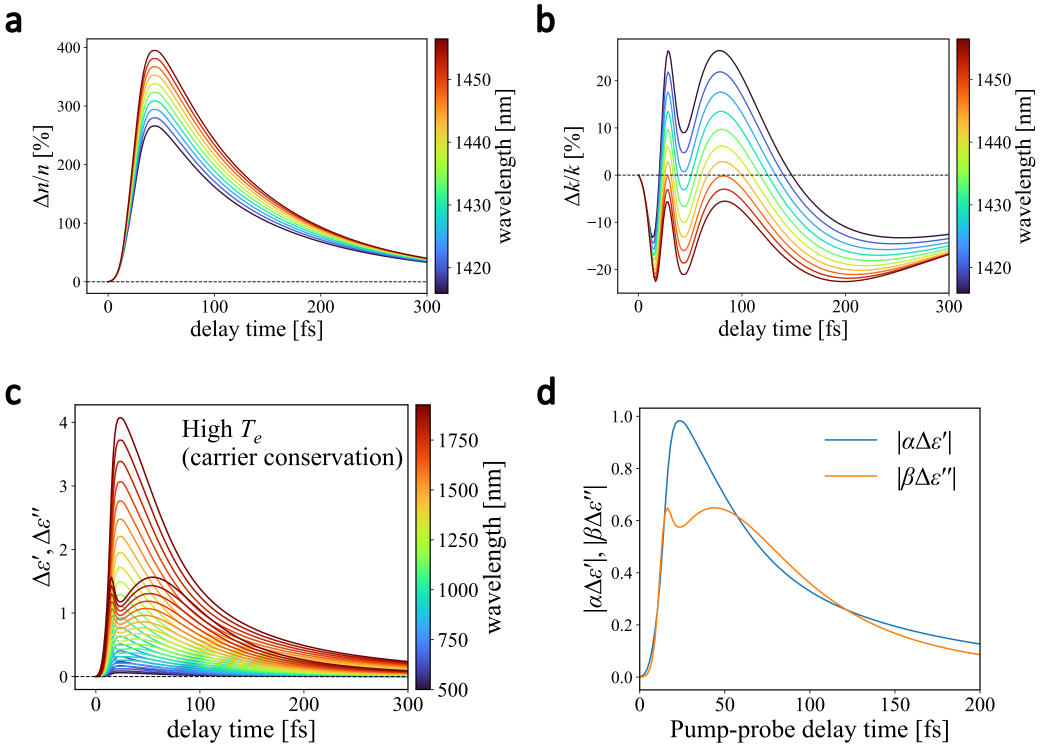


Figure S6: **a**, $\Delta n(\tau)/n$ of the absorber layer exhibiting a single-peaked response. **b**, $\Delta k(\tau)/k$ of the absorber layer showing oscillatory response. **c**, Real and imaginary permittivity modulation in the absorber layer. $\Delta\epsilon'$ shows a single peak response, while $\Delta\epsilon''$ exhibits oscillatory response. **d**, Absolute value of left and right term of Eq. S1 at near-ENZ probe wavelength (1437 nm), indicating the contribution of refraction and absorption on transmittance oscillation.

## 10 Spectral tunability of the zero-crossing through angular variation

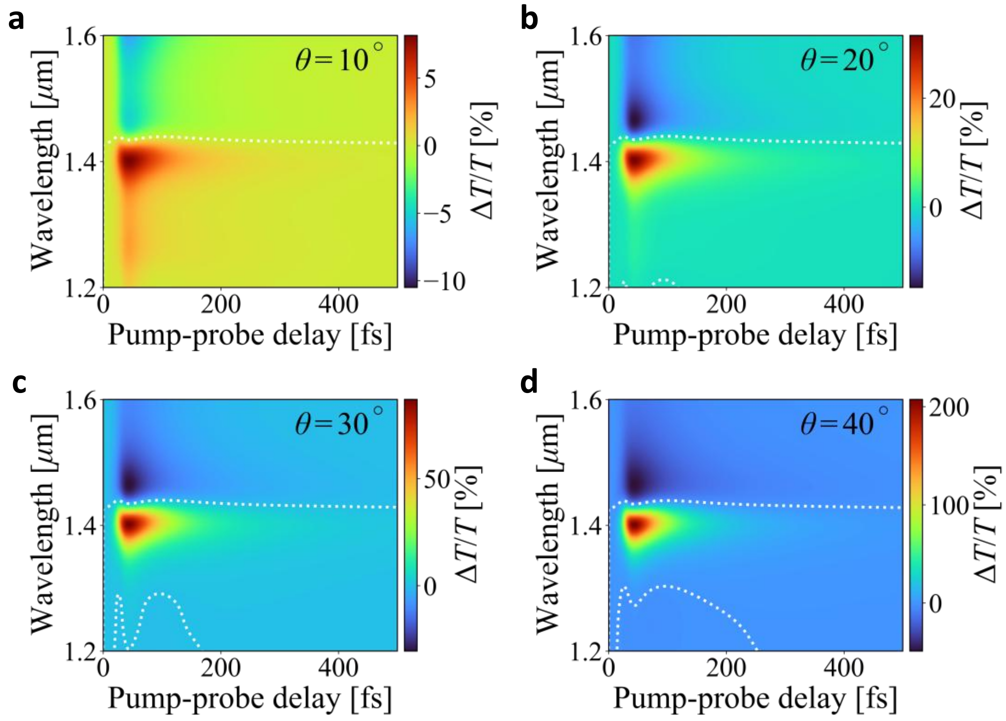


Figure S7: **Angular dependence of transmittance modulation under $p$-polarized probe.** $p$-polarized probe incident angle-dependent transmittance modulation as a function of pump–probe delay and wavelength, highlighting an effective spectral and temporal tunability of the zero-crossing. Dotted lines indicate the zero-crossing. **a**, 10°; **b**, 20°; **c**, 30°; **d**, 40°.

Figure S7 shows the transmittance modulation for various $p$-polarized probe incident angles. As the incident angle increases, the modulation strength increases due to the larger $z$-component in the incident electric field, which is strongly enhanced due to the ENZ boundary condition. In addition to amplitude tunability, the spectral and temporal range of the off-ENZ zero-crossing can be tuned through angular variation. Upon increasing the incident angle,

the zero-crossing redshifts, appearing within the range at 20°, while the oscillatory spectral range narrows after reaching its maximum at 30°. These trends show that the spectral location, temporal dynamics, and amplitude of the reversals can be actively controlled through angle tuning. However, the ENZ-associated zero-crossing region remains largely insensitive to angle variation, highlighting its intrinsic robustness.

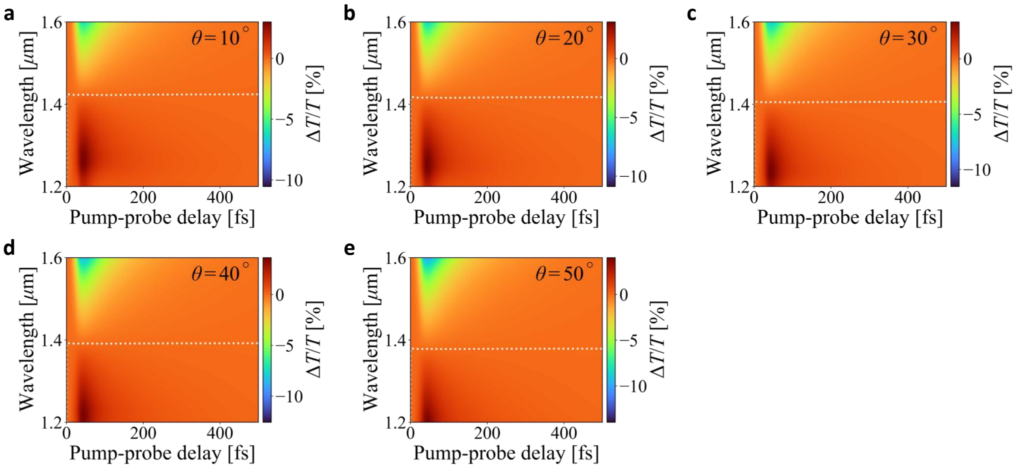


Figure S8: **Angular dependence of transmittance modulation under $s$-polarized probe.** $s$-polarized probe incident angle-dependent transmittance modulation as a function of pump–probe delay and wavelength. The modulation response remains largely unchanged with varying incident angle. Dotted lines indicate the spectral positions of the zero-crossing points. **a**, 10°; **b**, 20°; **c**, 30°; **d**, 40°; **e**, 50°.

Figure S8(a–e) shows the transmittance modulation under varying incident angles for an $s$-polarized probe beam. Apart from a slight blueshift in the zero-crossing positions (indicated by the dotted lines), the transmittance dynamics remain nearly identical across all probe incident angles. This contrasts with the pronounced $p$-polarization sensitivity and confirms that the oscillatory response is primarily probed by the $z$-component of the electric field, only accessible under $p$-polarized probe beam.

# 11 Absolute transmittance modulation spectrum

The absolute transmittance modulation clarifies the strong response near the ENZ region. The transmittance is close to zero near the ENZ range due to the strong cavity-enhanced ENZ absorption. This enables a large relative transmittance modulation, much stronger than that of a single 10-nm TCO film. This capability makes the multilayer cavity particularly attractive for high-performance optical switches, modulators, and sensing devices. Figure S9(a) shows the absolute transmission modulation as a function of wavelength. A pronounced dip appears near 1.5 $\mu$m, while a peak is observed around 1.4 $\mu$m. The transmittance spectra before ($T_1$) and after ($T_2$) modulation are presented in Figure S9(b), taken at the time of maximum electron temperature (42 fs after excitation). A peak and dip appear in the ($T_2$) spectrum centered around the ENZ wavelength (marked by the green dotted line). Notably, the dip region reaches near-zero transmittance, due to enhanced absorption.

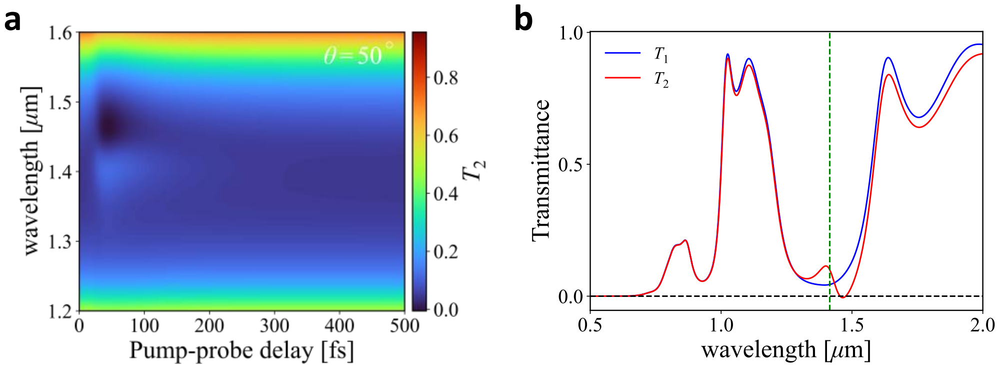


Figure S9: **a**, Absolute transmittance modulation as a function of pump–probe delay and wavelength. **b**, Absolute transmittance modulation spectrum at the delay time corresponding to the maximum electron temperature (42 fs), exhibiting an opposite behavior near the ENZ wavelength.

# 12 Electron temperature-dependent chemical potential and carrier density of the TCO absorber/acceptor layer

The dynamic carrier density modulation induced by thermionic carrier injection drives an oscillatory refractive index modulation in the TCO-based electron acceptor layer. Figure S7(a) and (b) present the carrier density and chemical potential calculated under the Sommerfeld approximation and a more realistic model with the varying carrier density calculated through thermionic emission theory, respectively. Figure S10(a) shows the increasing carrier density and suppressed chemical potential drop in the absorber layer (initial carrier density of $7.35 \times 10^{26}$ m$^{-3}$) under the Sommerfeld approximation. Figure S10(b) shows the increasing carrier density over electron temperature in the acceptor layer ($0.5 \times 10^{26}$ m$^{-3}$) calculated by the thermionic emission theory. The thermionically injected carrier density as a function of electron temperature is calculated using Eq. S18, assuming a 10 fs injection time at each temperature. The resemblance between the trend in (a) and (b) highlights that the mechanism of refractive oscillation can be reproduced by thermionic carrier injection.

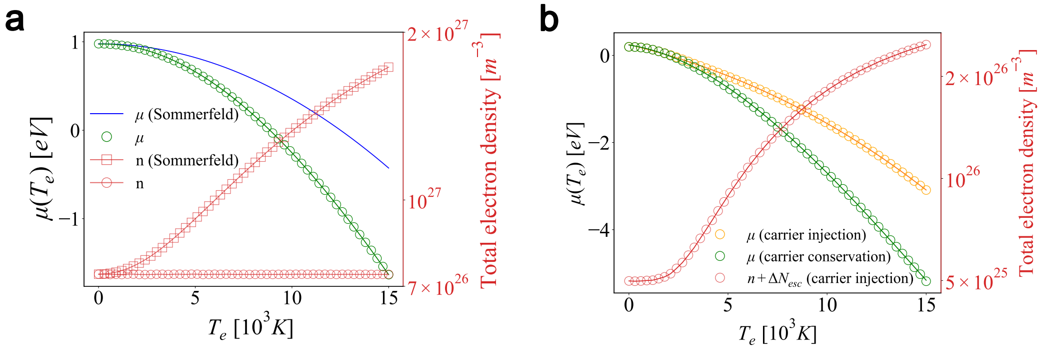


Figure S10: **a**, Total carrier density and chemical potential of the TCO absorber layer (initial carrier density of $7.35 \times 10^{26}$ m$^{-3}$) over electron temperature, under the Sommerfeld (blue) and carrier-conserving (red) models. The carrier density increases and exhibits a smaller chemical potential drop at elevated electron temperature. **b**, Total electron density and chemical potential in the TCO electron-acceptor layer (initial carrier density of $0.5 \times 10^{26}$ m$^{-3}$). The yellow and green dotted lines highlight the reduced chemical potential drop resulting from thermionic carrier injection.

# 13 Temporal and spectral tunability of $\Delta n/n$

The zero-crossing regions can be engineered by changing the carrier concentration of the acceptor layer. In Figure S11(a), the contour redshifts to longer wavelengths as the carrier concentration decreases, while the width of the contour region widens, resulting in a longer duration of the cycles. On the other hand, Figure S11(b) shows an additional control offered by changing the peak electron temperature with a fixed acceptor layer carrier concentration of $0.5 \times 10^{26}$ m$^{-3}$. Increasing the peak electron temperatures from 12,000 K to 20,000 K extends the zero-crossing region to the shorter wavelengths, further broadening the spectral range of oscillatory $\Delta n/n$ from NIR to visible. This analysis demonstrates the flexibility of the oscillatory dynamics and the benefits of driving the peak electron temperature to higher values.

The spectral position of the zero-crossing can be tuned not only by ad-

justing the carrier concentration and peak electron temperature but also through band-structure engineering, which can be controlled via microstructure and defect engineering during material processing. Such modifications alter the non-parabolic band structure, which is characterized by the conduction band minimum effective mass and the non-parabolicity parameter. The influence of these parameters on the zero-crossing is illustrated in Figure S11(c) and (d). As the effective mass increases from $0.2\,m_0$ to $0.6\,m_0$, the zero-crossing undergoes a blueshift, accompanied by narrowing temporal width. Interestingly, at $0.7\,m_0$, the zero-crossing shifts abruptly to a spectral region near $0.5\,\mu$m. Figure S11(d) shows the dependence of zero-crossing on non-parabolicity with a fixed conduction band minimum effective mass of $m^* = 0.24m_e$. Notably, a blueshift is observed in the zero-crossing spectral regions with increasing non-parabolicity. This effect originates from a stronger energy dependence of the effective mass upon increasing non-parabolicity, which abruptly alters the effective mass at higher energy levels.

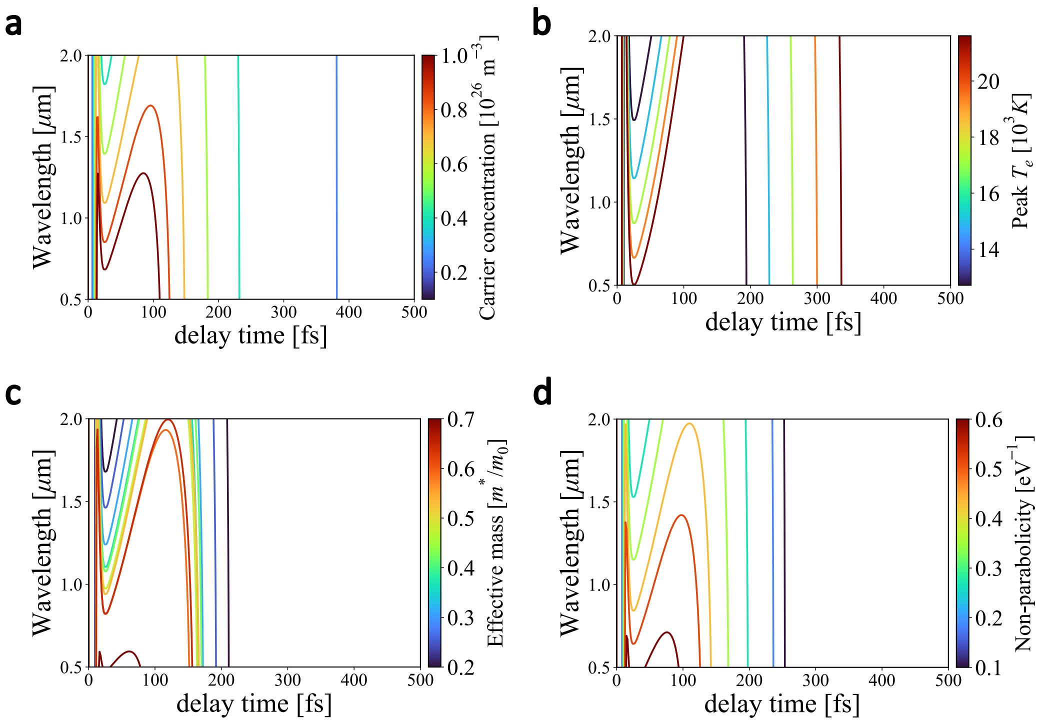


Figure S11: **a**, Zero-crossing contours of $\Delta n(\tau)/n$ across different acceptor layer carrier densities, highlighting the spectral and temporal tunability of the oscillatory dynamics. **b**, Zero-crossing contours of $\Delta n(\tau)/n$ over peak electron temperatures in the acceptor layer, showing an extended reversal range at higher $T_e$. **c**, Zero-crossing contours of $\Delta n(\tau)/n$ as a function of the conduction band minimum effective mass, $m_0^*$. **d**, Zero-crossing contours of $\Delta n(\tau)/n$ as a function of the non-parabolicity parameter.

# References

[1] Alam, M. Z., De Leon, I. & Boyd, R. W. Large optical nonlinearity of indium tin oxide in its epsilon-near-zero region. *Science* **352**, 795–797 (2016).

[2] Kinsey, N. *et al.* Epsilon-near-zero al-doped zno for ultrafast switching at telecom wavelengths. *Optica* **2**, 616–622 (2015).

[3] Afinogenov, B. I., Bessonov, V. O., Soboleva, I. V. & Fedyanin, A. A. Ultrafast all-optical light control with tamm plasmons in photonic nanostructures. *ACS Photonics* **6**, 844–850 (2019).

[4] Ashoka, A. *et al.* Extracting quantitative dielectric properties from pump-probe spectroscopy. *Nature Communications* **13**, 1437 (2022).

[5] Guo, P., Schaller, R. D., Ketterson, J. B. & Chang, R. P. Ultrafast switching of tunable infrared plasmons in indium tin oxide nanorod arrays with large absolute amplitude. *Nature Photonics* **10**, 267–273 (2016).

[6] Alam, M. Z., Schulz, S. A., Upham, J., De Leon, I. & Boyd, R. W. Large optical nonlinearity of nanoantennas coupled to an epsilon-near-zero material. *Nature Photonics* **12**, 79–83 (2018).

[7] Kahaly, M. U., Madas, S., Mesits, B. & Kahaly, S. Tunable ultrafast thermionic emission from femtosecond-laser hot spot on a metal surface by control of laser polarization and angle of incidence: A numerical investigation. *Applied Surface Science* **643**, 158668 (2024).

[8] Guo, J. *et al.* Simulation of thermionic emission optimization in femtosecond laser irradiation metal film by two-layer structure. *Applied Physics A* **117**, 1367–1374 (2014).

[9] Rethfeld, B., Kaiser, A., Vicanek, M. & Simon, G. Ultrafast dynamics of nonequilibrium electrons in metals under femtosecond laser irradiation. *Physical Review B* **65**, 214303 (2002).

[10] Uehlein, M. *et al.* Capturing non-equilibrium electron dynamics in metals accurately and efficiently. *arXiv preprint arXiv:2503.09479* (2025).

[11] Baxter, J. *et al.* Understanding the nonlinear optical response of epsilon near zero materials in the time-domain. *arXiv preprint arXiv:2110.14806* (2021).

[12] Chang, H.-T. *et al.* Electron thermalization and relaxation in laser-heated nickel by few-femtosecond core-level transient absorption spectroscopy. *Physical Review B* **103**, 064305 (2021).

[13] de Roulet, B. R., Drescher, L., Sato, S. A. & Leone, S. R. Initial electron thermalization in metals measured by attosecond transient absorption spectroscopy. *Physical Review B* **110**, 174301 (2024).

[14] Sarkar, S., Un, I. W. & Sivan, Y. Electronic and thermal response of low-electron-density drude materials to ultrafast optical illumination. *Physical Review Applied* **19**, 014005 (2023).

[15] O'Keeffe, P. *et al.* Ultrafast dynamics of nonthermal carriers following plasmonic and interband photoexcitation of 2d arrays of gold nanoparticles. *ACS Photonics* **11**, 3205–3212 (2024).
